# Supplementary material for: Ultrafast structural dynamics of the Fe-pnictide parent compound BaFe2As2
Source: arXiv:1411.0718 source file (2014-11-03)
Supplement: Supplementary file 1 [file Rettig_BaFe2As2_Slicing_Supplement_subm.pdf]

# Supplemental material to: Ultrafast structural dynamics of the Fe-pnictide parent compound $BaFe_2As_2$

L. Rettig,[1] S. O. Mariager,[1] A. Ferrer,[2,1] S. Grübel,[1] J. A. Johnson,[1] J. Rittmann,[3,1] T. Wolf,[4] S. L. Johnson,[2] G. Ingold,[1,5] P. Beaud,[1,5] and U. Staub[1]

[1]*Swiss Light Source, Paul Scherrer Institut, CH-5232 Villigen PSI, Switzerland*

[2]*Institute for Quantum Electronics, Physics Department, ETH Zürich, CH-8093 Zürich, Switzerland*

[3]*Ecole Polytechnique Fédérale de Lausanne, Laboratoire de Spectroscopie Ultrarapide, ISIC, FSB, CH-1015 Lausanne, Switzerland*

[4]*Karlsruhe Institute of Technology, Institut für Festkörperphysik, D-76021 Karlsruhe, Germany*

[5]*SwissFEL, Paul Scherrer Institut, CH-5232 Villigen PSI, Switzerland*

(Dated: November 3, 2014)

## STRUCTURE FACTOR CALCULATIONS

In the kinematic approximation, the x-ray diffraction intensity is proportional to the structure factor squared,

$$I(\mathbf{G}) \propto |F(\mathbf{G})|^2 = \left| \sum_{\text{u.c.}} f_n^G e^{i\mathbf{r_n}\cdot\mathbf{G}} \right|^2 \quad , \tag{S1}$$

where $\mathbf{G}$ is the reciprocal lattice vector and $f_n^G$ and $\mathbf{r_n}$ are the atomic form factor and atom position of the $n$-th atom in the unit cell. The structure of $BaFe_2As_2$ [1] yields for the two reflections

$$F_{105}(z) = f_{\text{Ba}}^{105} + 2f_{\text{As}}^{105} \cdot \cos(2\pi \cdot 5z) \tag{S2}$$

$$F_{206}(z) = f_{\text{Ba}}^{206} - 2f_{\text{Fe}}^{206} + 2f_{\text{As}}^{206} \cdot \cos(2\pi \cdot 6z) \quad , \tag{S3}$$

where $z$ is the As coordinate along the crystal's $c$ axis, which directly depends on the Fe-As tetrahedra angle $\alpha$ by $z(\alpha) = 0.25 + 0.152\tan(\alpha)$. The calculated diffraction intensities for the two reflections including the x-ray polarization factor $P$ are shown in Fig. S1 as a function of tetrahedra angle $\alpha$. The relative intensities at the equilibrium position, $I_{(105)}/I_{(206)} \approx 1.6$ agree reasonably well with the experimental intensities (see fig. 1 of the main manuscript), justifying the use of the kinematic approximation.

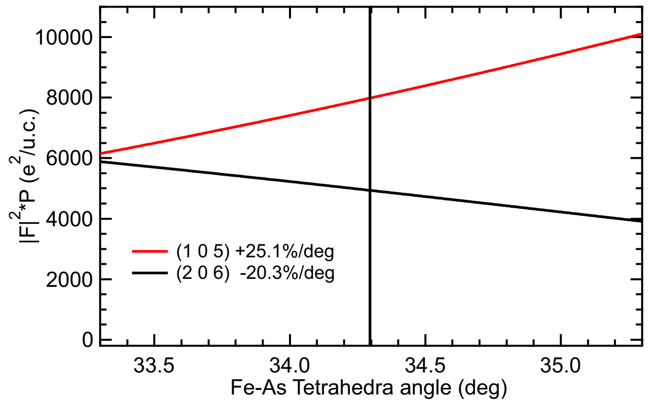


FIG. S1. Calculated diffraction intensity for the (1 0 5) (red) and (2 0 6) (black) reflections as a function of the Fe-As tetrahedra angle $\alpha$.

## DEPENDENCE ON THE PROBE PENETRATION DEPTH

In order to compare the oscillation and displacement amplitudes to the time-resolved photoemission data, the different probe depths of the photoemission and the x-ray experiments have to be taken into account. For the two investigated reflections, the outgoing diffracted beam leaves at an angle $\beta \sim 30-45$ deg to the surface, allowing constructive interference of the outgoing x-ray beams from different probe depths [2]. The diffracted intensity can then be written as:

$$I \propto \left| \int_0^\infty F(\zeta) \cdot e^{-\zeta/2\lambda_{\mathrm{xray}}} \mathrm{d}\zeta \right|^2 \quad , \tag{S4}$$

where $\lambda_{\mathrm{xray}}$ is the x-ray penetration depth perpendicular to the surface at the grazing incidence angle. Here, the absorption of the outgoing diffracted beam has been neglected. The inhomogeneous excitation due to the laser absorption length $\lambda_{\mathrm{laser}}$ leads to a dependence of the structure factor $F(\zeta)$ with the distance $\zeta$ from the surface, where the displacement is assumed to be linear with pump fluence:

$$F(\zeta) = F(z_0 + \Delta z \cdot e^{-\zeta/\lambda_{\mathrm{laser}}}) \quad , \tag{S5}$$

with $z_0$ the equilibrium As coordinate and $\Delta z$ the (fluence and time-dependent) As displacement amplitude at the surface.

The photoelectron escape depth at the kinetic energy $E_{\mathrm{kin}} \sim 20$ eV in the experiments by Yang et *al.* [3] is on the order of 10 Å $\ll \lambda_{\mathrm{laser}}$, and thus measures the coherent oscillation

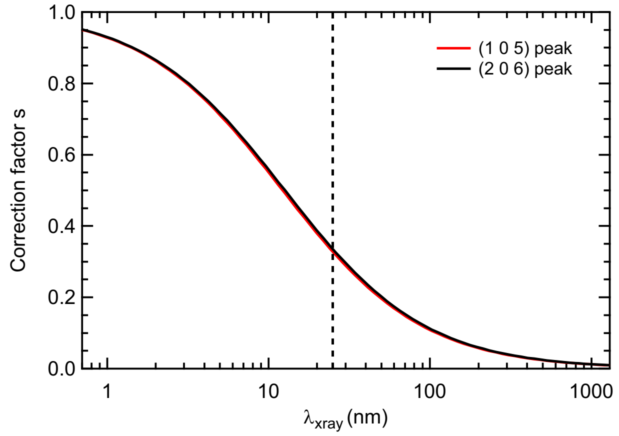


FIG. S2. Correction factor $s$ as function of x-ray penetration depth $\lambda_{\mathrm{xray}}$, for $\lambda_{\mathrm{laser}} = 25$ nm, and for a displacement amplitude $\Delta z = 2 \times 10^{-3}$ ($\Delta\alpha = 0.5$ deg). The dashed line marks the x-ray penetration depth $\lambda_{\mathrm{xray}} = 25$ nm used in the experiment.

amplitudes at the surface. Equation (S4) has been calculated as a function of x-ray penetration depth $\lambda_{\mathrm{xray}}$ for the two reflections, yielding a correction factor $s = \Delta z_{\mathrm{avg}}/\Delta z_{\mathrm{surface}}$, which is shown in Fig. S2. For the experimental value of $\lambda_{\mathrm{xray}} = 25\,\mathrm{nm}$, we obtain $s \approx \frac{1}{3}$, which is taken into account to calculate the deformation potential.


[1] M. Rotter, M. Tegel, and D. Johrendt, Phys. Rev. Lett. **101**, 107006 (2008).

[2] P. Beaud, A. Caviezel, S. O. Mariager, L. Rettig, G. Ingold, C. Dornes, S.-W. Huang, J. A. Johnson, M. Radovic, T. Huber, T. Kubacka, A. Ferrer, H. T. Lemke, M. Chollet, D. Zhu, J. M. Glownia, M. Sikorski, A. Robert, H. Wadati, M. Nakamura, M. Kawasaki, Y. Tokura, S. L. Johnson, and U. Staub, Nat. Mater. **13**, 923 (2014).

[3] L. X. Yang, G. Rohde, T. Rohwer, A. Stange, K. Hanff, C. Sohrt, L. Rettig, R. Cortés, F. Chen, D. L. Feng, T. Wolf, B. Kamble, I. Eremin, T. Popmintchev, M. M. Murnane, H. C. Kapteyn, L. Kipp, J. Fink, M. Bauer, U. Bovensiepen, and K. Rossnagel, Phys. Rev. Lett. **112**, 207001 (2014).
